# Supplementary material for: A Distributed Edge FLISR Solution & Network Simulation Test Platform
Source: arXiv:2407.17497 source file (2024-07-05)
Supplement: Supplementary file 1 [file appendix_a.tex]

\begin{table*}[!hbp]
\vspace{0.5cm}
    \centering
    \caption{\label{table:3}Centralised FLISR algorithm correlated results}
    \begin{adjustbox}{width=\textwidth}
    \begin{tabular}{lllllllllp{5cm}}
    \toprule
        Start time & End time & Faulted devices & Down devices & Operation & \parbox{2cm}{Affected customers pre operation} & \parbox{2cm}{Affected customers post operation} & \parbox{2cm}{CML per hour pre operation} & \parbox{2cm}{CML per hour post operation} \\ [0.1cm]
    \midrule
        2023-09-02 13:18:45.519 & 2023-09-02 13:18:45.726 & \parbox{2cm}{S507} & \parbox{3cm}{S508, R518, S509, S697} & \parbox{7cm}{S507 opened, S508 closed, R518 closed, S509 closed, S697 N/O point closed} & 1370 & 0 & 78090 & 0 \\ [0.5cm]
        2023-09-02 13:27:35.724 & 2023-09-02 13:27:35.916 & \parbox{2cm}{S507, S508} & \parbox{3cm}{R518, S509, S697} & \parbox{7cm}{S507 opened, S508 opened, R518 closed, S509 closed, S697 N/O point closed} & 1370 & 171 & 78090 & 9747 \\
        2023-09-02 13:30:09.237 & 2023-09-02 13:30:09.413 & \parbox{2cm}{S507, S508, R518, S509} & \parbox{3cm}{S697} & \parbox{7cm}{S507 opened, S508 opened, R518 opened, S509 opened, S697 N/O point closed} & 1370 & 1136 & 78090 & 64752 \\ [0.5cm]
        2023-09-02 13:31:06.018 & 2023-09-02 13:31:06.168 & \parbox{2cm}{S696, S699} & \parbox{3cm}{S698, S510, S697} & \parbox{7cm}{S696 opened, S699 opened, S698 closed, S510 closed, S697 N/O point closed} & 152 & 102 & 8664 & 5814 \\ [0.5cm]
        2023-09-02 13:31:27.330 & 2023-09-02 13:31:27.512 & \parbox{2cm}{R517} & \parbox{3cm}{S513, S512, S716, S700, S514} & \parbox{7cm}{R517 opened, S513 closed, S512 closed, S716 closed, S700 N/O point closed, S514 N/O point closed} & 784 & 0 & 44688 & 0 \\ [0.5cm]
        2023-09-02 13:32:02.604 & 2023-09-02 13:32:02.785 & \parbox{2cm}{R517, S513} & \parbox{3cm}{S512, S700, S716, S514} & \parbox{7cm}{R517 opened, S513 opened, S512 closed, S700 N/O point closed, S716 closed, S514 N/O point closed} & 784 & 157 & 44688 & 8949 \\ [0.5cm]
        2023-09-02 13:33:33.993 & 2023-09-02 13:33:34.173 & \parbox{3cm}{R517, S513, S512, S716, S700} & \parbox{3cm}{S514} & \parbox{7cm}{R517 opened, S513 opened, S512 closed, S700 N/O point closed, S716 closed, S514 N/O point closed} & 784 & 756 & 44688 & 43092 \\ [0.5cm]
        2023-09-02 13:34:20.536 & 2023-09-02 13:34:20.766 & \parbox{2cm}{S515, S511} & \parbox{3cm}{S510, S514, S698, S697, S699} & \parbox{7cm}{S515 N/O point opened, S511 opened, S510 closed, S514 N/O point closed, S698 closed, S697 N/O point closed, S699 closed} & 1136 & 1038 & 64752 & 59166 \\ [0.5cm]
        2023-09-02 13:35:04.120 & 2023-09-02 13:35:04.260 & \parbox{2cm}{R830, R799} & \parbox{3cm}{R797} & \parbox{7cm}{R830 opened, R799 opened, R797 N/O point closed} & 812 & 380 & 46284 & 21660 \\ [0.5cm]
        2023-09-02 13:35:51.775 & 2023-09-02 13:35:51.928 & \parbox{2cm}{R830} & \parbox{3cm}{R799, R797} & \parbox{7cm}{R830 opened, R799 closed, R797 N/O point closed} & 812 & 0 & 46284 & 0 \\ [0.5cm]
        2023-09-02 13:36:31.083 & 2023-09-02 13:36:31.232 & \parbox{2cm}{R794} & \parbox{3cm}{R798, R795, R796, R797} & \parbox{7cm}{R794 opened, R798 closed, R795 closed, R796 closed, R797 N/O point closed} & 1065 & 0 & 60705 & 0 \\ [0.5cm]
        2023-09-02 13:37:10.572 & 2023-09-02 13:37:10.718 & \parbox{2cm}{R794, R798} & \parbox{3cm}{R795, R796, R797} & \parbox{7cm}{R794 opened, R798 opened, R795 closed, R796 closed, R797 N/O point closed} & 1065 & 156 & 60705 & 8892 \\ [0.5cm]
        2023-09-02 13:37:52.575 & 2023-09-02 13:37:52.718 & \parbox{2cm}{R794, R798, R795} & \parbox{3cm}{R796, R797} & \parbox{7cm}{R794 opened, R798 opened, R795 opened, R796 closed, R797 N/O point closed} & 1065 & 406 & 60705 & 23142 \\ [0.5cm]
        2023-09-02 13:38:31.922 & 2023-09-02 13:38:32.067 & \parbox{2cm}{R794, R798, R795, R796} & \parbox{3cm}{R797} & \parbox{7cm}{R794 opened, R798 opened, R795 opened, R796 opened, R797 N/O point closed} & 1065 & 724 & 60705 & 41268 \\ [0.5cm]
        2023-09-02 13:39:27.791 & 2023-09-02 13:39:27.975 & \parbox{2cm}{R183, S175} & \parbox{3cm}{R184, R181, R182} & \parbox{7cm}{R183 opened, S175 opened, R184 N/O point closed, R181 N/O point closed, R182 N/O point closed} & 426 & 320 & 24282 & 18240 \\ [0.5cm]
        2023-09-02 13:40:31.084 & 2023-09-02 13:40:31.244 & \parbox{2cm}{R186} & \parbox{3cm}{R185, R184} & \parbox{7cm}{R186 opened, R185 closed, R184 N/O point closed} & 250 & 0 & 14250 & 0 \\ [0.5cm]
        2023-09-02 13:41:05.087 & 2023-09-02 13:41:05.231 & \parbox{2cm}{R186, R185} & \parbox{3cm}{R184} & \parbox{7cm}{R186 opened, R185 opened, R184 N/O point closed} & 250 & 83 & 14250 & 4731 \\ [0.5cm]
    \bottomrule
    \end{tabular}
    \end{adjustbox}
\end{table*}

\begin{table*}[!ht]
\vspace{0.5cm}
    \centering
    \caption{\label{table:4}Distributed FLISR algorithm correlated results}
    \begin{adjustbox}{width=\textwidth}
    \begin{tabular}{lllllllllp{5cm}}
    \toprule
        Start time & End time & Faulted devices & Down devices & Operation & \parbox{2cm}{Affected customers pre operation} & \parbox{2cm}{Affected customers post operation} & \parbox{2cm}{CML per hour pre operation} & \parbox{2cm}{CML per hour post operation} \\ [0.1cm]
    \midrule
        2023-09-02 13:20:16.366 & 2023-09-02 13:20:16.368 & \parbox{2cm}{S507} & \parbox{3cm}{S508, R518, S509, S697} & \parbox{7cm}{S507 opened, S508 closed, R518 closed, S509 closed, S697 N/O point closed} & 2740 & 171 & 156180 & 9747 \\ [0.5cm]
        2023-09-02 13:30:25.304 & 2023-09-02 13:30:25.306 & \parbox{2cm}{S507, S508, R518} & \parbox{3cm}{S509, S697} & \parbox{7cm}{S507 opened, S508 opened, R518 opened, S509 closed, S697 N/O point closed} & 1370 & 844 & 78090 & 48108 \\ [0.5cm]
        2023-09-02 13:31:45.643 & 2023-09-02 13:31:45.646 & \parbox{2cm}{R517} & \parbox{3cm}{S513, S512, S700, S716, S514} & \parbox{7cm}{R517 opened, S513 closed, S512 closed, S700 N/O point closed, S716 closed, S514 N/O point closed} & 784 & 0 & 44688 & 0 \\ [0.5cm]
        2023-09-02 13:32:21.187 & 2023-09-02 13:32:21.189 & \parbox{2cm}{R517, S513} & \parbox{3cm}{S512, S716, S514, S700} & \parbox{7cm}{R517 opened, S513 opened, S512 closed, S716 closed, S514 N/O point closed, S700 N/O point closed} & 784 & 157 & 44688 & 8949 \\ [0.5cm]
        2023-09-02 13:33:51.724 & 2023-09-02 13:33:51.726 & \parbox{2cm}{R517, S513, S512, S700, S716} & \parbox{3cm}{S514} & \parbox{7cm}{R517 opened, S513 opened, S512 opened, S700 N/O point opened, S716 opened, S514 N/O point closed} & 784 & 479 & 44688 & 27303 \\ [0.5cm]
        2023-09-02 13:34:44.674 & 2023-09-02 13:34:44.677 & \parbox{2cm}{S515, S511} & \parbox{3cm}{S510, S514, S698, S699, S697} & \parbox{7cm}{S515 N/O point opened, S511 opened, S510 closed, S514 N/O point closed, S698 closed, S699 closed, S697 N/O point closed} & 1136 & 1038 & 64752 & 59166 \\ [0.5cm]
        2023-09-02 13:35:19.620 & 2023-09-02 13:35:19.622 & \parbox{2cm}{R830, R799} & \parbox{3cm}{R797} & \parbox{7cm}{R830 opened, R799 opened, R797 N/O point closed} & 812 & 380 & 46284 & 21660 \\ [0.5cm]
        2023-09-02 13:36:12.840 & 2023-09-02 13:36:12.841 & \parbox{2cm}{R830} & \parbox{3cm}{R799, R797} & \parbox{7cm}{R830 opened, R799 closed, R797 N/O point closed} & 812 & 0 & 46284 & 0 \\ [0.5cm]
        2023-09-02 13:36:51.611 & 2023-09-02 13:36:51.614 & \parbox{2cm}{R794} & \parbox{3cm}{R798, R795, R796, R797} & \parbox{7cm}{R794 opened, R798 closed, R795 closed, R796 closed, R797 N/O point closed} & 1065 & 0 & 60705 & 0 \\ [0.5cm]
        2023-09-02 13:37:30.684 & 2023-09-02 13:37:30.687 & \parbox{2cm}{R794, R798} & \parbox{3cm}{R795, R796, R797} & \parbox{7cm}{R794 opened, R798 opened, R795 closed, R796 closed, R797 N/O point closed} & 1065 & 156 & 60705 & 8892 \\ [0.5cm]
        2023-09-02 13:38:11.829 & 2023-09-02 13:38:11.831 & \parbox{2cm}{R794, R798, R795} & \parbox{3cm}{R796, R797} & \parbox{7cm}{R794 opened, R798 opened, R795 opened, R796 closed, R797 N/O point closed} & 1065 & 406 & 60705 & 23142 \\ [0.5cm]
        2023-09-02 13:38:51.291 & 2023-09-02 13:38:51.293 & \parbox{2cm}{R794, R798, R795, R796} & \parbox{3cm}{R797} & \parbox{7cm}{R794 opened, R798 opened, R795 opened, R796 opened, R797 N/O point closed} & 1065 & 724 & 60705 & 41268 \\ [0.5cm]
        2023-09-02 13:39:52.897 & 2023-09-02 13:39:52.900 & \parbox{2cm}{R198, R183} & \parbox{3cm}{R184, S175, R182, R181} & \parbox{7cm}{R198 opened, R183 opened, R184 N/O point closed, S175 closed, R182 N/O point closed, R181 N/O point closed} & 589 & 163 & 33573 & 9291 \\ [0.5cm]
        2023-09-02 13:40:48.348 & 2023-09-02 13:40:48.350 & \parbox{2cm}{R186} & \parbox{3cm}{R185, R184} & \parbox{7cm}{R186 opened, R185 closed, R184 N/O point closed} & 250 & 0 & 14250 & 0 \\ [0.5cm]
        2023-09-02 13:41:21.393 & 2023-09-02 13:41:21.394 & \parbox{2cm}{R186, R185} & \parbox{3cm}{R184} & \parbox{7cm}{R186 opened, R185 opened, R184 N/O point closed} & 250 & 83 & 14250 & 4731 \\ [0.5cm]
    \bottomrule
    \end{tabular}
    \end{adjustbox}
\end{table*}
% subsection appendix_a (end)
